# Supplementary material for: Growth and Structure of Singly-Oriented Single-Layer Tungsten Disulfide on Au(111)
Source: arXiv:1806.04928 source file (2018-09-19)
Supplement: Supplementary file 1 [file Bignardi_PRM_Supplementary.pdf]

# Growth and Structure of Singly-Oriented Single-Layer Tungsten Disulfide on Au(111). Supplementary Material

Luca Bignardi,[1] Daniel Lizzit,[1] Harsh Bana,[2] Elisabetta Travaglia,[2] Paolo Lacovig,[1] Charlotte E. Sanders,[3] Maciej Dendzik,[3,*] Matteo Michiardi,[3] Marco Bianchi,[3] Moritz Ewert,[4,5] Lars Buß,[4] Jens Falta,[4,5] Jan Ingo Flege,[4,5] Alessandro Baraldi,[1,2,6] Rosanna Larciprete,[7] Philip Hofmann,[3,†] and Silvano Lizzit[1,‡]

[1]*Elettra - Sincrotrone Trieste S.C.p.A., AREA Science Park, Strada Statale 14, km 163.5, 34149 Trieste, Italy.*

[2]*Department of Physics, University of Trieste, Via Valerio 2, 34127 Trieste, Italy.*

[3]*Department of Physics and Astronomy, Interdisciplinary Nanoscience Center (iNANO), Aarhus University, Ny Munkegade 120, 8000 Aarhus C, Denmark.*

[4]*Institute of Solid State Physics, University of Bremen, Otto-Hahn-Allee 1, 28359 Bremen, Germany*

[5]*MAPEX Center for Materials and Processes, Bremen, Germany*

[6]*IOM-CNR, Laboratorio TASC, AREA Science Park, Strada Statale 14, km 163.5, 34149 Trieste, Italy.*

[7]*CNR-Institute for Complex Systems, Via dei Taurini 19, 00185 Roma, Italy.*

[*] Current address: Department of Physical Chemistry, Fritz-Haber-Institut of the Max Planck Society, Faradayweg 4-6, Berlin 14915, Germany.

[†] philip@phys.au.dk

[‡] lizzit@elettra.eu

## I. LINESHAPE OF CORE LEVELS

| Au $4f_{7/2}$ ($h\nu$=136 eV) | $L$(eV) | $\alpha$ | G(eV) | SCLS(eV) |
|---|---|---|---|---|
| Bulk (B) | 0.31 | 0.02 | 0.09 | 0.0 |
| Surface ($S_{clean}$) | 0.37 | 0.02 | 0.23 | -0.33 |
| $Au_{WS_2}$ | 0.37 | 0.02 | 0.23 | -0.09 |

TABLE I. Line shape parameters for different components in the Au $4f_{7/2}$ spectrum acquired at 136 eV photon energy. $L$ is the Lorentzian width, $\alpha$ is the asymmetry parameter and G is the Gaussian width.

## II. DETERMINATION OF THE $WS_2$ COVERAGE

In figure 1 the high-resolution XPS spectra of the Au $4f_{7/2}$ core level are shown for the clean Au(111) (top) and after the growth of $WS_2$ for GR2. Table I presents the parameters of the peaks fitting. After the growth of SL $WS_2$ an extra component ($Au_{WS_2}$) appears and it is accompanied by the decrease in the intensity of the clean surface peak $Au_S$. This new peak can be attributed to the Au surface atoms in direct contact with the $WS_2$ layer. In

| W $4f$ ($h\nu$=140 eV) | $L$(eV) | $\alpha$ | G(eV) | BE(eV) |
|---|---|---|---|---|
| $4f_{7/2}$ | 0.13 | 0.01 | 0.08 | 32.79 |
| $4f_{5/2}$ | 0.16 | 0.01 | 0.09 | 34.93 |
| S $2p$ ($h\nu$=260 eV) | $L$(eV) | $\alpha$ | G(eV) | BE(eV) |
| $2p_{3/2}$ $S_A$ | 0.18 | 0.03 | 0.15 | 162.45 |
| $2p_{3/2}$ $S_B$ | 0.22 | 0.02 | 0.21 | 162.59 |
| $2p_{1/2}$ $S_A$ | 0.18 | 0.03 | 0.15 | 163.65 |
| $2p_{1/2}$ $S_B$ | 0.22 | 0.02 | 0.21 | 163.79 |

TABLE II. Line shape parameters for different components for W 4f and S 2p spectra acquired at 140 eV and 260 eV photon energy, respectively, for growth GR2. $L$ is the Lorentzian width, $\alpha$ is the asymmetry parameter and G is the Gaussian width. The main peaks for GR1 have the same lineshape and BE position.

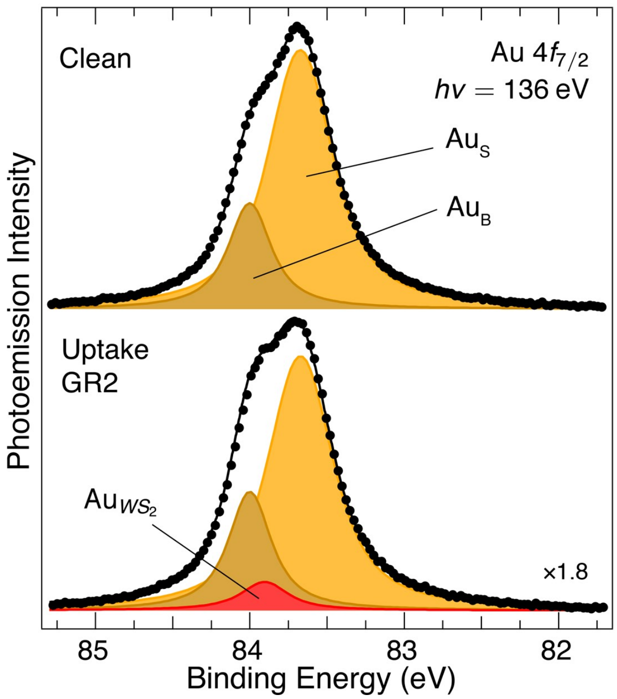


FIG. 1. Au $4f_{7/2}$ component measured for clean Au surface (top) and after growth GR2 (bottom). The photon energy was 136 eV.

order to calculate the $WS_2$ coverage we considered the decrease of the $Au_S$ component in the Au $4f_{7/2}$ spectrum after $WS_2$ growth for the sample prepared with GR2, where only the $WS_2$ related XPS features are present. The coverage $\theta$ can be extracted from

$$\theta_{WS_2}(t) = 1 - \frac{I_{AuS}(t)}{I_{AuS}(t=0)}, \tag{1}$$

where $I_{AuS}(t)$ indicates the intensity of the surface component of Au 4f at time $t$. We find for GR2 a $WS_2$ coverage of 45%. The same $WS_2$ coverage was present at the end of uptake GR1 as found by comparing the intensity of the blue W $4f$ components in Figure 3b and d.

## III. ORIENTATION OF THE AU SUBSTRATE

The orientation of the Au(111) surface is necessary to identify the relative stacking of the $WS_2$ layer on the substrate. This information was obtained performing XPD measurements of the Au $4f_{7/2}$ core level for the clean sample, as mentioned in the main text. Figure 2a and 2c show the XPD patterns corresponding to the bulk ($Au_B$) and clean surface ($Au_S$) components (colored), respectively, measured at 400 eV photon energy (photoelectron kinetic

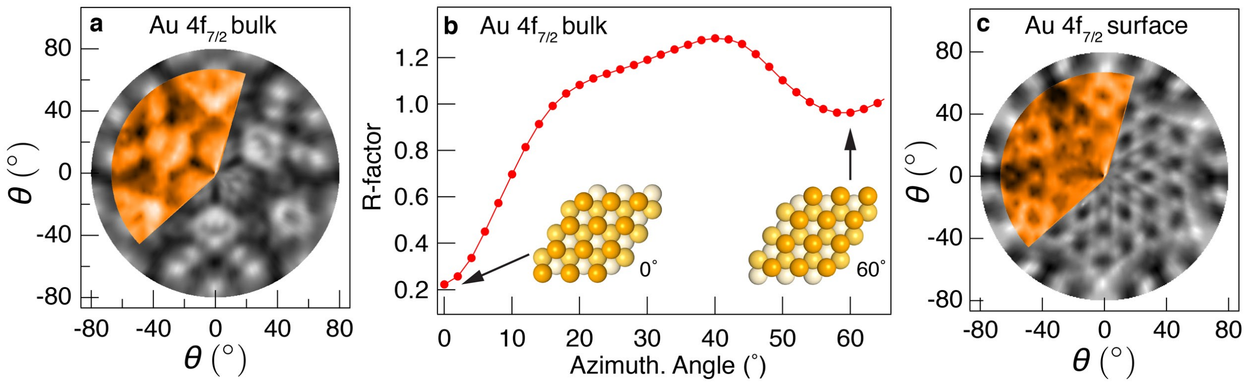


FIG. 2. XPD pattern acquired at 400 eV photon energy (KE∼316 eV), showing the XPD pattern (color) associated to the bulk component $Au_B$ (a) and to the surface component $Au_S$ (c) of the Au $4f_{7/2}$ core level together with the multiple scattering simulation (grey) for the clean Au(111) sample with the azimuthal orientation of 0° depicted in (b). (b) R-factor vs azimuthal angle for the XPD pattern associated to the bulk peak of the Au $4f_{7/2}$.

energy∼ 316 eV). The expected three-fold symmetry is observed for the XPD pattern of the bulk component, while the herringbone reconstruction returns an almost six-fold symmetric pattern for the $4f_{7/2}$ surface component $Au_S$. Therefore, the XPD pattern of the bulk peak was used to determine the orientation of the Au substrate. The pattern for the bulk component was simulated with a bulk-terminated surface, accounting for the high absolute value of the R-factor. The herringbone reconstruction was simulated by compressing the surface unit cell in the $\langle -110 \rangle$ direction by 4.5%, averaging over the three 60° rotated domains, while three layers below the surface were considered as the bulk. In order to unambiguously identify the orientation of the substrate, we performed an R-factor analysis calculating the XPD patterns of the bulk peak for different azimuthal orientations of the Au(111) substrate. The analysis (Figure 2b) shows the absolute minimum of the R-factor (0.2) for the substrate orientation corresponding to an azimuthal angle of 0°, i.e. with the same orientation of the model depicted in Figure 2b.

## IV. FAST-XPS CHARACTERIZATION OF $WS_2$ GROWTH

In Figure 3a and b, a fast-XPS intensity plot is shown together with the peak fit analysis of the last W $4f_{7/2}$ core level spectrum of the fast-XPS spectral sequence for GR1. The

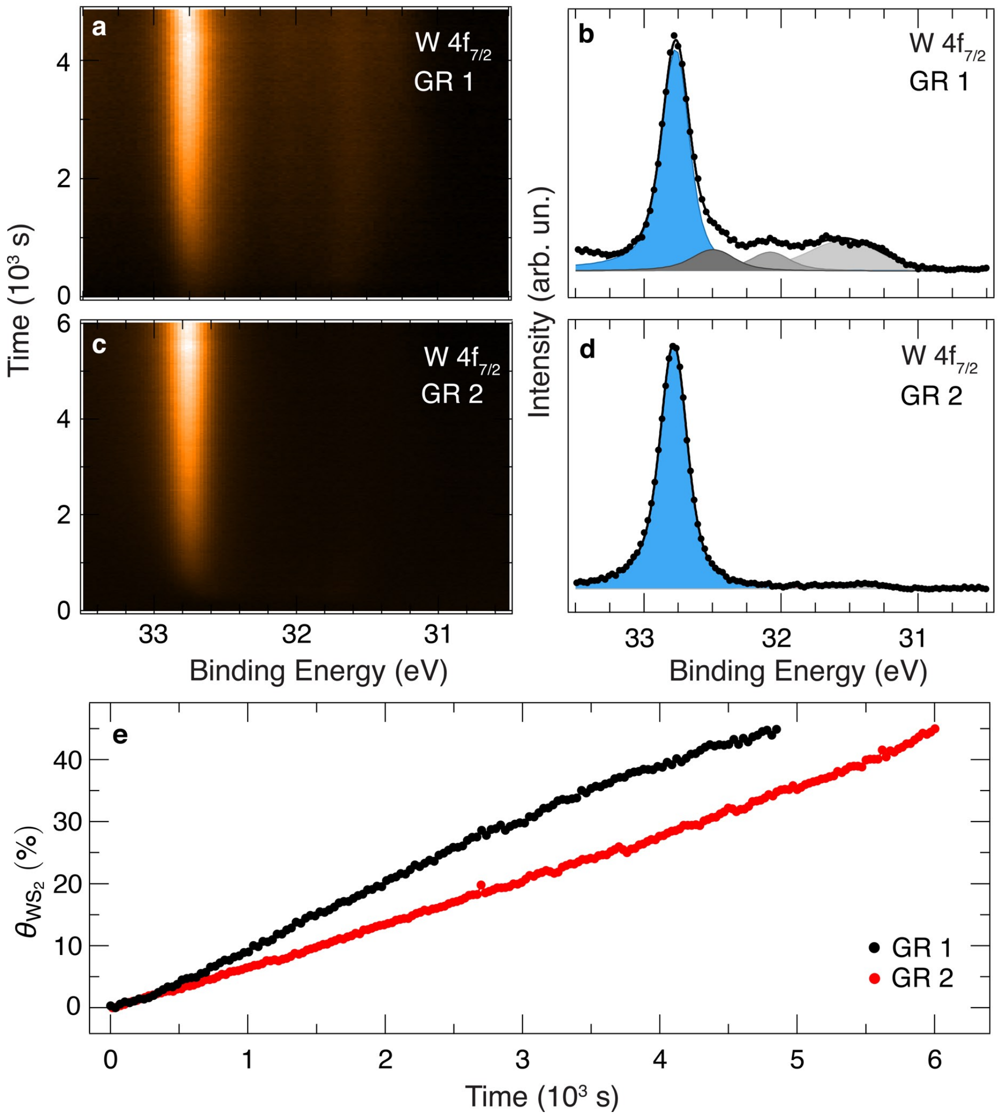


FIG. 3. (a) and (c) W $4f_{7/2}$ fast-XPS intensity plot obtained for GR1 and GR2, respectively, together with the last W $4f_{7/2}$ core level spectra of the fast-XPS series (b and d), showing the spectral contributions resulting from peak fit analysis. The photon energy is 140 eV. (e) Evolution of the $WS_2$ coverage in time for the two growths.

growth of the peak at a binding energy (BE) BE=32.79 eV (blue) corresponding to $WS_2$ is accompanied by the contribution from various components at lower BE [1]. The presence of these components is consistent with the formation of incompletely sulfided species of the form $WS_{2-x}$, (with $0 < x \leq 1$), as observed for the same system in earlier literature [1, 2]. In Figure 3c and d we show the results achieved on GR2. For this growth, only the component

associated with $WS_2$ is observed.

The coverage of $WS_2$ ($\theta_{WS_2}$), which is proportional to the intensity of the main blue component of the W $4f$ core level, is shown as a function of time for both uptakes in Figure 3e. $\theta_{WS_2}$ was calculated from the intensity loss of the clean surface peak of the Au $4f_{7/2}$ XPS spectra after the growth of the $WS_2$ layer (Figure 1). In Figure 3e we observe that the $\theta_{WS_2}$ is an almost linear function of the W deposition time for GR2 (red curve) throughout the deposition, up to a $WS_2$ coverage of about 45%. This suggests that all the deposited W atoms react and form $WS_2$. On the contrary, the $\theta_{WS_2}$ obtained for GR1 shows a deviation from the linear behavior, with a modification of the slope around a coverage of 25%. Moreover, the much higher W deposition rate for GR1 (more than double than that for Growth 2) is not reflected in a comparable increase of the $WS_2$ growth rate, as seen from the slope of the two curves in the initial stage of the growth. This is due to the formation of incompletely sulfided species right from the beginning which, as the coverage increases, prevent the formation of $WS_2$.

## V. DETERMINATION OF THE POLYTYPE

X-ray photoelectron diffraction is an excellent tool to determine the polytype of the $WS_2$ monolayers on Au(111). This goal is achieved by measuring the XPD patterns from the bottom component of the S $2p_{3/2}$ core level, i.e. the component associated to S atoms in direct contact with the Au substrate, and choosing a photon energy ($h\nu = 560$ eV) tuned to enhance the forward scattering conditions. In this way, we can map the positions of the scattering atoms (mainly W), with respect to the S emitter. These experimental patterns are reported in Figure 4 together with simulated patterns sourcing from a trigonal prismatic (1H) structure (Figure 4a) and from octahedral (1T) structure (Figure 4b and c). Two distinct mirrored 1T structures were simulated, similarly to the two possible orientations that the 1H structure can assume. A sketch of the simulated structures is shown at the top of the figure. The results obtained performing a R-factor analysis (see the main text for details) are R=0.24 for the 1H structure and R=1.23 and R=0.66 for the two 1T structures. The minimum R-factor observed for the patterns shown in Figure 4a is clearly indicative of a 1H structure. The good agreement between simulations and experiments corroborates the fact that the component at higher BE observed for each of the spin-split peaks of the

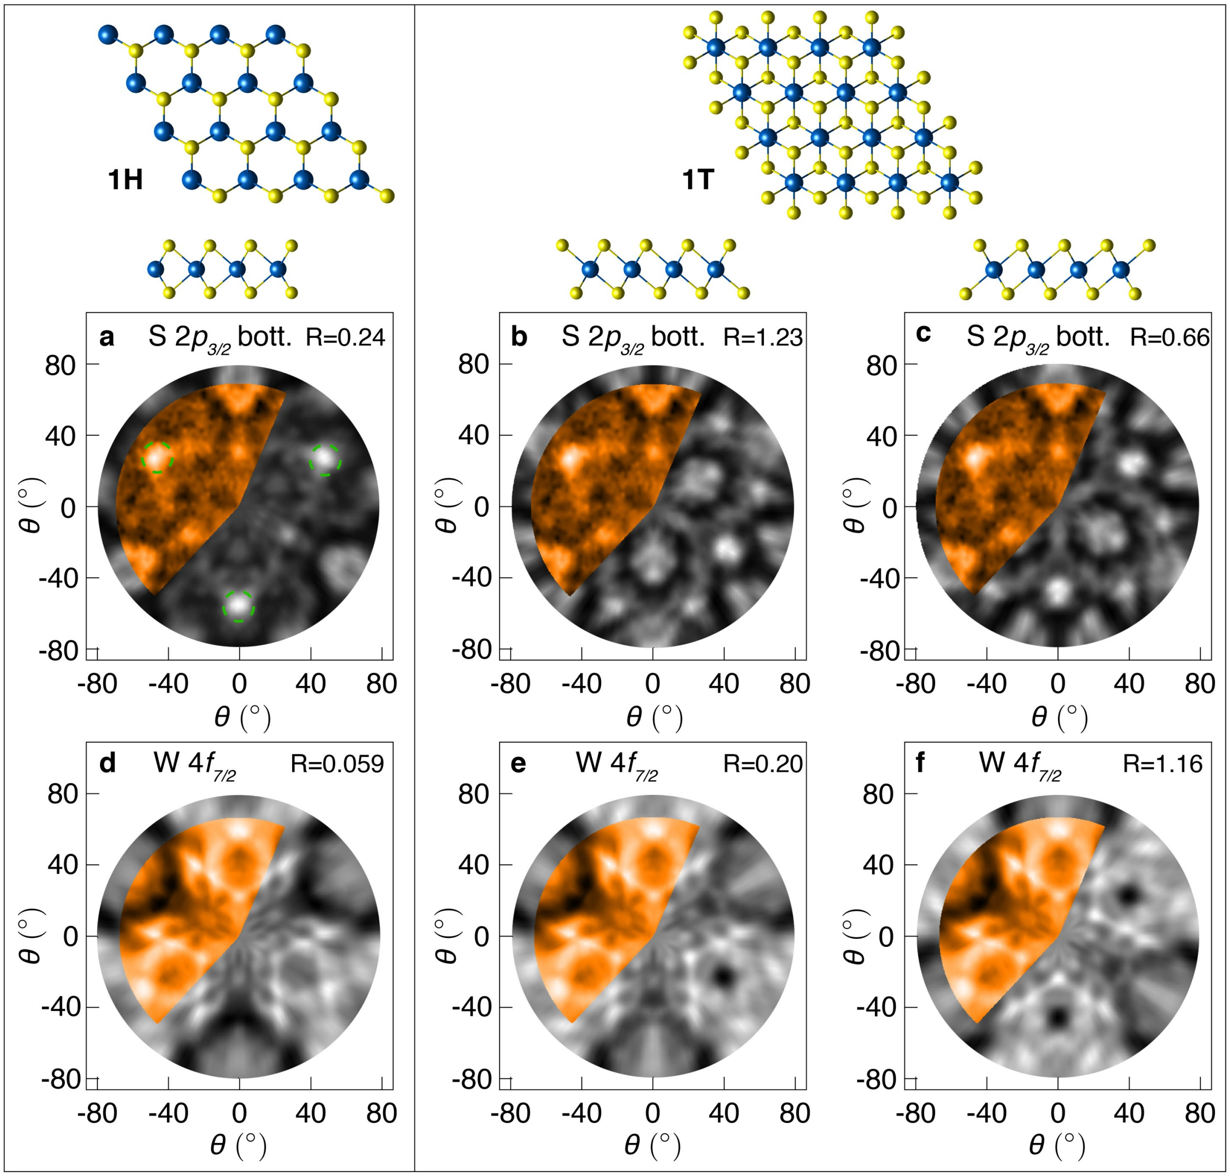


FIG. 4. Determination of the polytype of $WS_2$ layer. The XPD experimental patterns (colored sector) obtained for bottom S $2p_{3/2}$ component (acquired at $h\nu = 560$ eV) are compared with simulations performed for the 1H (a) and for the two 1T polytypes (b and c), as depicted at the top of the figure. Similar results but W $4f_{7/2}$ are displayed in the bottom row (acquired at $h\nu = 170$ eV). The green circles indicate the position of the forward-scattering peaks due to the W atoms.

S $2p_{3/2}$ spectrum originates from the bottom sulfur layer. The higher absolute value of the R-factor obtained for the pattern of $S_{\mathrm{bottom}}$ –when compared to the case of W $4f_{7/2}$– depends on the small photoemission signal from the bottom sulfur atoms, worsening the statistics

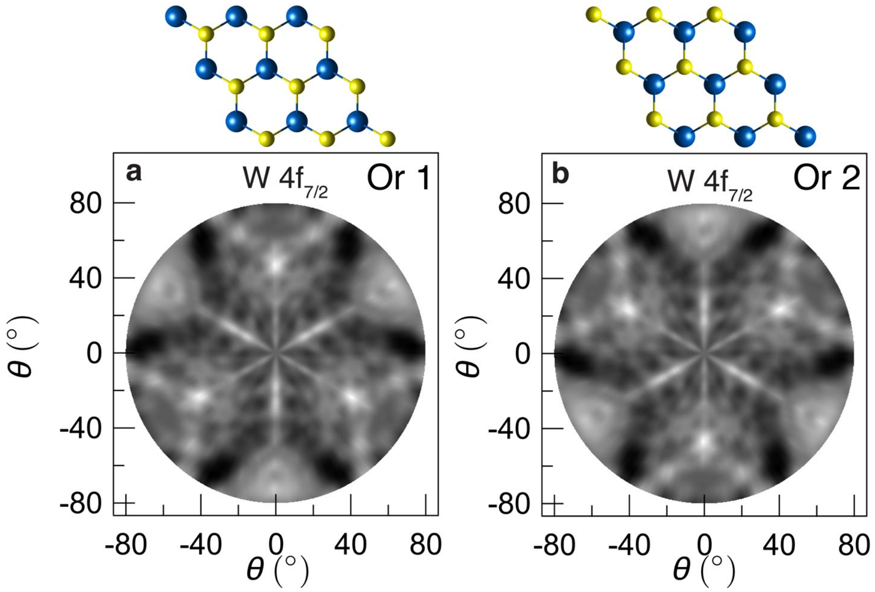


FIG. 5. $WS_2$ atomic ball model for the main and mirror domains with the corresponding XPD simualtions. As expected there is a mere rotation of 60° or, equivalently 180° between the two XPD patterns. Simulations performed by using the lattice parameters that minimize the R-factor in Figure 2 of the main text.

and signal-to-noise ratio of the measurement. On the other hand, the quality of the data is sufficient to observe clearly the forward-scattering peaks due to the W scatterers in the layer.

A similar experiment and comparison has been carried out for the W $4f_{7/2}$ core level, acquired with a photon energy of 160 eV, for which both forward and backward scattering processes are present. The R-factor minimization returns an R-factor of 0.059, 0.20 and 1.16, respectively, validating the outcomes observed for S 2p and showing unambiguously that $WS_2$ assumes the 1H polytype structure on the Au(111) surface.

## VI. SIMULATED XPD PATTERNS FOR MIRROR ORIENTATION

An important information that can be extracted from XPD is the detection of mirror domains in the $WS_2$ layer. Some information about the domain orientation can be readily obtained from a mere inspection of the diffraction pattern without any need for simulations. If, for instance, there is an equal area covered by the two mirror domains, the diffraction

pattern would be expected to show a sixfold symmetry. If, on the other hand, only one orientation is present, the symmetry should be three-fold. Such simple arguments are only valid when the (threefold) Au(111) substrate is neglected in the calculations but this turns out to be a valid approximation due to the absence of the same local arrangement of the $WS_2$ atoms with respect to the Au atoms because of the mismatch between the two lattices.

Figure 5(a) and (b) show simulated W $4f_{7/2}$ XPD patterns for the two mirrored orientations (labeled Or1 and Or2, respectively) for a free-standing $WS_2$ layer with 1H geometry as depicted in the ball-model at the top. These patterns are calculated for an electron kinetic energy (KE) of 326 eV. Since the Au(111) substrate is neglected in these simulations, the diffraction patterns are identical although mirrored.

## VII. $\mu$LEED OF $WS_2$ DOMAINS

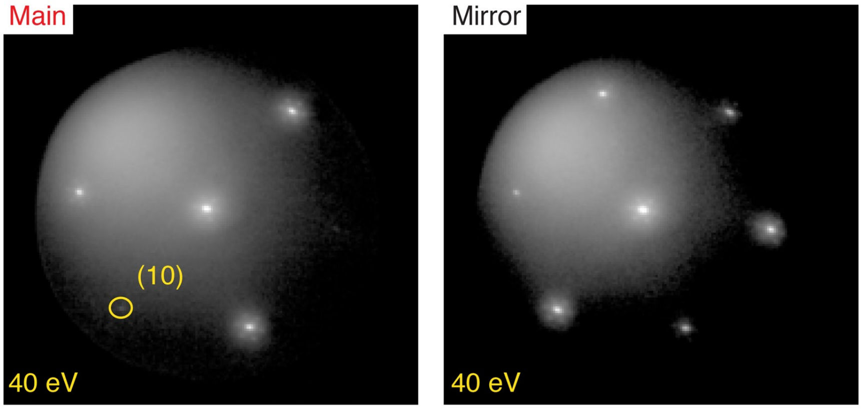


FIG. 6. μLEED patterns acquired on the main and mirror SL $WS_2$ domains, as labelled in the main text, for the same electron energy (40 eV).

As explained in the main text, we could identify the presence of a negligible amount of SL $WS_2$ domains assuming the mirror, $W_{hcp}S_{top}$ configuration, which are minority with respect to the main $W_{fcc}S_{top}$ configuration (see Figure 6c and 6d). The two orientations can be seen in a μLEED experiment, as shown in Figure 6. The two patterns show a three-fold symmetry, which is reversed in between them. This indicates that the patterns are produced

by mirrored structures.

---

[1] Maciej Dendzik, Matteo Michiardi, Charlotte Sanders, Marco Bianchi, Jill A. Miwa, Signe S. Grønborg, Jeppe V. Lauritsen, Albert Bruix, Bjørk Hammer, and Philip Hofmann, "Growth and electronic structure of epitaxial single-layer $WS_2$ on au(111)," Phys. Rev. B **92**, 245442 (2015).

[2] Henrik G. Fuchtbauer, Anders K. Tuxen, Poul G. Moses, Henrik Topsoe, Flemming Besenbacher, and Jeppe V. Lauritsen, "Morphology and atomic-scale structure of single-layer $WS_2$ nanoclusters," Phys. Chem. Chem. Phys. **15**, 15971–15980 (2013).
